# Supplementary material for: Markov property of Lagrangian turbulence
Source: arXiv:2104.03136 ancillary file (2022-06-24)
Supplement: Supplementary file 1 [file SuppMaterial.pdf]

# Supplementary material: The entropy and fluctuation theorems of inertial particles in turbulence

A. FUCHS<sup>1</sup>, M. OBLIGADO<sup>2</sup>, M. BOURGOIN<sup>3</sup>, M. GIBERT<sup>4</sup>, P.D. MININNI<sup>5</sup> and J. PEINKE<sup>1</sup>

<sup>1</sup> *Institute of Physics and ForWind, University of Oldenburg, Küppersweg 70, 26129 Oldenburg, Germany*

<sup>2</sup> *Univ. Grenoble Alpes, CNRS, Grenoble INP\*, LEGI, 38000 Grenoble, France*

<sup>3</sup> *Laboratoire de Physique de l'École Normale Supérieure de Lyon, CNRS & Université de Lyon, 46 allée d'Italie, F-69364 Lyon Cedex 07, France*

<sup>4</sup> *Univ. Grenoble Alpes, CNRS, Grenoble INP, Institut Néel, 38000 Grenoble, France*

<sup>5</sup> *Universidad de Buenos Aires, Facultad de Ciencias Exactas y Naturales, Departamento de Física, & IFIBA, CON-ICET, Ciudad Universitaria, Buenos Aires 1428, Argentina*

**Abstract** –This document present the supplementary material on the research article: The entropy and fluctuation theorems of inertial particles in turbulence.

*Appendix A: Friedrich-Peinke approach.*— The evolution of the stochastic variable  $u_r$  possesses a Markov process “evolving” in  $r$ .  $u_r$  satisfies a diffusion process [1]

$$-\partial_r u_r = D^{(1)}(u_r, r) + [D^{(2)}(u_r, r)]^{1/2} \Gamma(r). \quad (1)$$

Due to the Markov assumption, the noise term  $\Gamma(r)$  is a random variable sampled from a zero-mean, white-noise Gaussian distribution with a variance of 2 and rapidly decaying correlations, such that  $\delta$ -correlation in scale can be assumed as  $\langle \Gamma(r) \Gamma(r') \rangle = 2\delta(r - r')$ .

The two functions  $D^{(1,2)}$  defining the Fokker-Planck equation are called drift and diffusion coefficients, respectively, and are defined by the two first conditional moments ( $k = 1, 2$ ,  $\tau' < \tau$  and  $\Delta\tau = \tau - \tau'$ )

$$M^{(k)}(u_\tau, \tau, \Delta\tau) = \int_{-\infty}^{\infty} (u_{\tau'} - u_\tau)^k p(u_{\tau'} | u_\tau) du_{\tau'}, \quad (2)$$

known as Kramers-Moyal coefficients:

$$D^{(k)}(u_\tau, \tau) = \lim_{\tau' \rightarrow \tau} \frac{M^{(k)}(u_\tau, \tau, \Delta\tau)}{k! (\tau' - \tau)}. \quad (3)$$

$D^{(k)}$  can be estimated directly from experimental data by an optimization procedure proposed in [2–5], which includes reconstruction of the conditional probability density functions  $p(u_{\tau'} | u_\tau)$ , based on approximating the solution of the corresponding Fokker-Planck equation using the short time propagator [6]. Similarly to previous works, [4, 5, 7–9] we use a linear function for  $D^{(1)}$  and a parabolic

function for  $D^{(2)}$  interpreted in the Itô convention [1]

$$D^{(1)}(u_\tau, \tau) = d_{11}(\tau) u_\tau, \quad (4)$$

$$D^{(2)}(u_\tau, \tau) = d_{22}(\tau) u_\tau^2 + d_{21}(\tau) u_\tau + d_{20}(\tau). \quad (5)$$

The estimated coefficients  $d_{ij}(\tau)$  are functions of scale  $\tau$  of the form  $\alpha(\tau/\tau_\eta)^\beta + \gamma$  (see Table 1-3 for details). The scale-dependent coefficients are estimated using an open-source Matlab package [10] and plotted in Fig. 1.

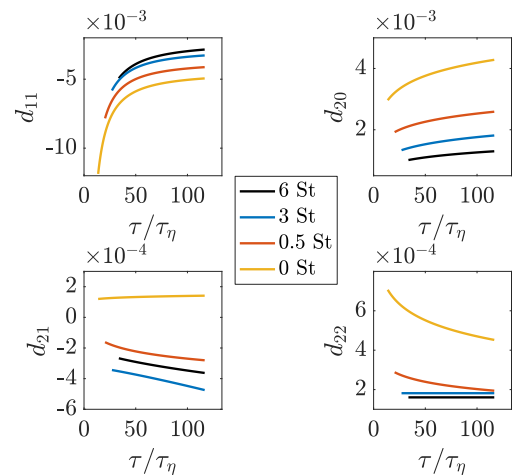

Fig. 1: Coefficients  $d_{ij}(\tau)$  of the Kramers-Moyal coefficients using the surface fits with a linear function for  $D^{(1)}(u_\tau, \tau)$  and a parabolic function for  $D^{(2)}(u_\tau, \tau)$  (see Eq. (4) - (5)) with respect to scale. Shown are coefficients  $d_{ij}(\tau)$  for  $x$  velocity component for all Stokes numbers considered ( $St = 0.5, 3$  and  $6$ ).

Table 1:  $\alpha$  of the coefficients  $d_{ij}(\tau)$  for all Stokes numbers considered ( $St = 0, 0.5, 3$  and  $6$ ).

|          | $St = 0$             | $St = 0.5$          | $St = 3$              | $St = 6$              |
|----------|----------------------|---------------------|-----------------------|-----------------------|
| $d_{11}$ | $\alpha = -2$        | $\alpha = -2$       | $\alpha = -2$         | $\alpha = -2$         |
| $d_{20}$ | $\alpha = 0.2676$    | $\alpha = 0.3015$   | $\alpha = 9.595e-05$  | $\alpha = 3.357e-10$  |
| $d_{21}$ | $\alpha = 9.859e-05$ | $\alpha = -1.2e-07$ | $\alpha = -7.179e-08$ | $\alpha = -0.0006$    |
| $d_{22}$ | $\alpha = 0.0094$    | $\alpha = -9.0e-04$ | $\alpha = 9.0884e-05$ | $\alpha = 8.1909e-05$ |

Table 2:  $\beta$  of the coefficients  $d_{ij}(\tau)$  for all Stokes numbers considered ( $St = 0, 0.5, 3$  and  $6$ ).

|          | $St = 0$          | $St = 0.5$        | $St = 3$          | $St = 6$          |
|----------|-------------------|-------------------|-------------------|-------------------|
| $d_{11}$ | $\beta = -1.2703$ | $\beta = -1.1690$ | $\beta = -1.2818$ | $\beta = -1.3818$ |
| $d_{20}$ | $\beta = 0.0023$  | $\beta = 0.0023$  | $\beta = 0.3704$  | $\beta = 1.8005$  |
| $d_{21}$ | $\beta = 0.0693$  | $\beta = 1.1790$  | $\beta = 1.1706$  | $\beta = 0.0955$  |
| $d_{22}$ | $\beta = -0.0137$ | $\beta = -0.1158$ | $\beta \approx 0$ | $\beta \approx 0$ |

**Appendix B: Probability density function of the total entropy variation  $S_{tot}$ .**— In order to observe the convergence of the exponential average to the theoretical value (integral fluctuation theorem), the occurrence of a sufficient number of realizations with  $\Delta S_{tot} < 0$  are crucial and therefore, the applications of fluctuation theorems are dependent on reliable statistics of rare events. In Fig. 2 the probability density function of the total entropy variation is plotted for  $x$  velocity component for all Stokes numbers considered ( $St = 0.5, 3$  and  $6$ ). This Figure shows that the entropy consuming trajectories with  $\Delta S_{tot} < 0$  occur frequently for all Stokes numbers.

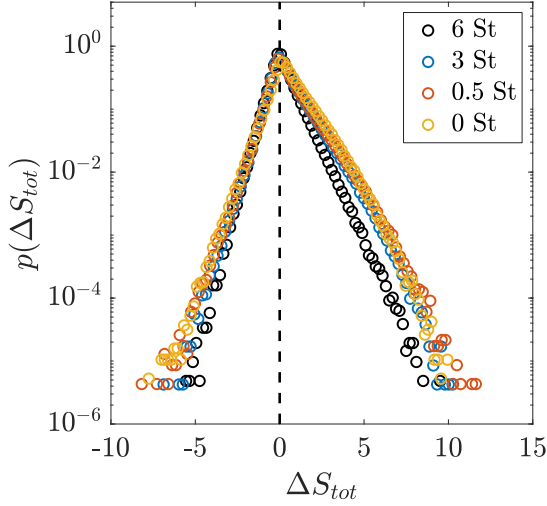
Fig. 2: Probability density function of the total entropy variation  $S_{tot}$  for all Stokes numbers considered ( $St = 0.5, 3$  and  $6$ ).

**Appendix C: Probability density function of the velocity increments  $u_\tau$ .**— In Figure 3 the probability density functions of velocity increments  $u_\tau/\sigma_\tau$  is plotted for the Lagrangian tracers with  $St = 0$ , for  $\Delta\tau = 3.5, 7, 14, 28\tau_\eta$ . The dashed line indicates a Gaussian distribution. The values of the kurtosis of the Lagrangian velocity increments, that quantify the deviation from the Gaussian, are additionally indicated in the legend. The two relevant values  $\Delta\tau$  are for  $7\tau_\eta$  and  $14\tau_\eta$ , as those are the upper and lower bounds that are mentioned in the manuscript.

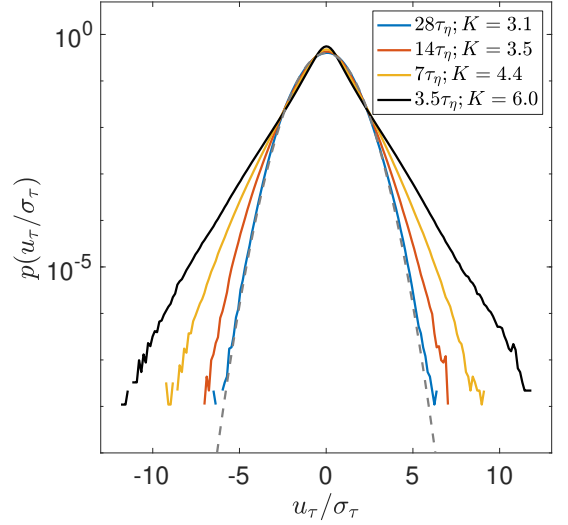
Fig. 3: PDF of the velocity increments  $u_\tau/\sigma_\tau$  for the Lagrangian tracers with  $St = 0$ , for  $\Delta\tau = 3.5, 7, 14, 28\tau_\eta$ . The grey dashed lines correspond to Gaussian fits.

Figure 4 shows the PDF of the velocity increments at the initial  $T \approx 120\tau_\eta$  and the time scale  $\Delta_{EM} \approx 13\tau_\eta$  for  $St = 3$ . In particular, the PDF at  $\Delta_{EM}$  is clearly different from a Gaussian distribution. Compared to the PDF's presented in Fig. 5 the statistics for the inertial particles become more Gaussian, as particles tend to filter the extreme events.

Table 3:  $\gamma$  of the coefficients  $d_{ij}(\tau)$  for all Stokes numbers considered ( $St = 0, 0.5, 3$  and  $6$ ).

|          | $St = 0$              | $St = 0.5$          | $St = 3$              | $St = 6$              |
|----------|-----------------------|---------------------|-----------------------|-----------------------|
| $d_{11}$ | $\gamma = -0.0045$    | $\gamma = -0.0019$  | $\gamma = -0.0028$    | $\gamma = -0.0028$    |
| $d_{20}$ | $\gamma = -0.2673$    | $\gamma = -0.3032$  | $\gamma = 0.0007$     | $\gamma = 0.0011$     |
| $d_{21}$ | $\gamma = -1.384e-05$ | $\gamma = -9.2e-05$ | $\gamma = -0.0003$    | $\gamma = 0.0007$     |
| $d_{22}$ | $\gamma = -0.0081$    | $\gamma = -2.2e-04$ | $\gamma = 9.0884e-05$ | $\gamma = 9.0884e-05$ |

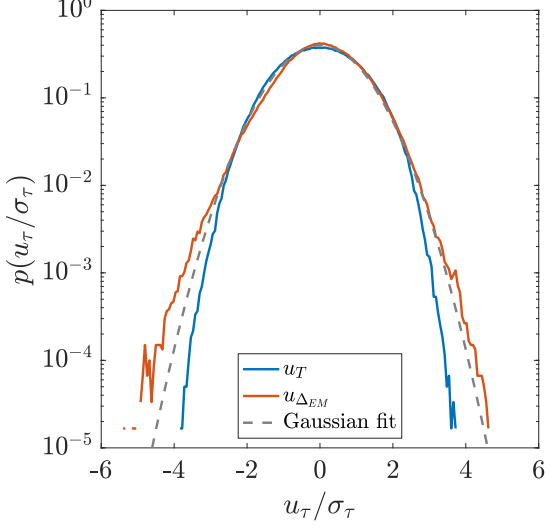
 Fig. 4: PDF of the velocity increments  $u_\tau$  at the initial  $T \approx 120\tau_\eta$  and the time scale  $\Delta_{EM} \approx 13\tau_\eta$  for  $St = 3$ . The grey dashed lines correspond to Gaussian fits.

*Appendix D: Kurtosis.*— Figure 5 shows the Kurtosis of velocity increments as a function of the timelag  $\Delta\tau$  (a) divided by the  $St$ -dependent critical time separation  $\Delta_{EM}$  and (b) divided by the Kolmogorov times  $\tau_\eta$  (defined as  $\tau_\eta = (\nu/\epsilon)^{1/2}$ ) for all  $St$  number cases.

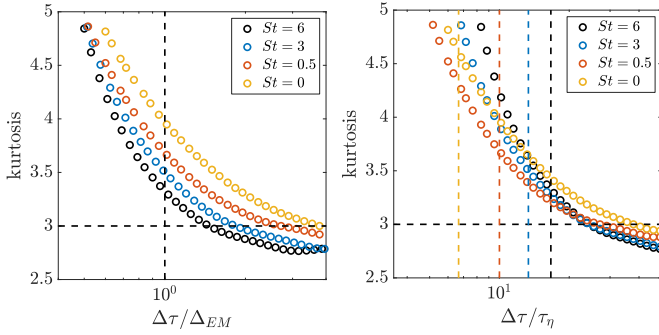
 Fig. 5: Kurtosis of velocity increments as a function of the time-lag  $\Delta\tau$  (a) divided by the  $St$ -dependent critical time separation  $\Delta_{EM}$  and (b) divided by the Kolmogorov times  $\tau_\eta$  (defined as  $\tau_\eta = (\nu/\epsilon)^{1/2}$ ) for all of our  $St$  number cases. The vertical dashed lines corresponds to the  $\Delta_{EM}$ .

This analysis demonstrates that on the scale that the Markov property holds the non-Gaussian behavior is still present.

*Appendix E: Increment PDFs conditioned on entropy.*—

In the following the condition on entropy and the influence on the statistics of increments on  $\Delta_{EM}$  is examined for  $St = 3$ . In Figure 6 the influence on the histogram (a) and the percentage proportion in relation to the full (no condition) data set (b) at  $\Delta_{EM}$  scale is presented.

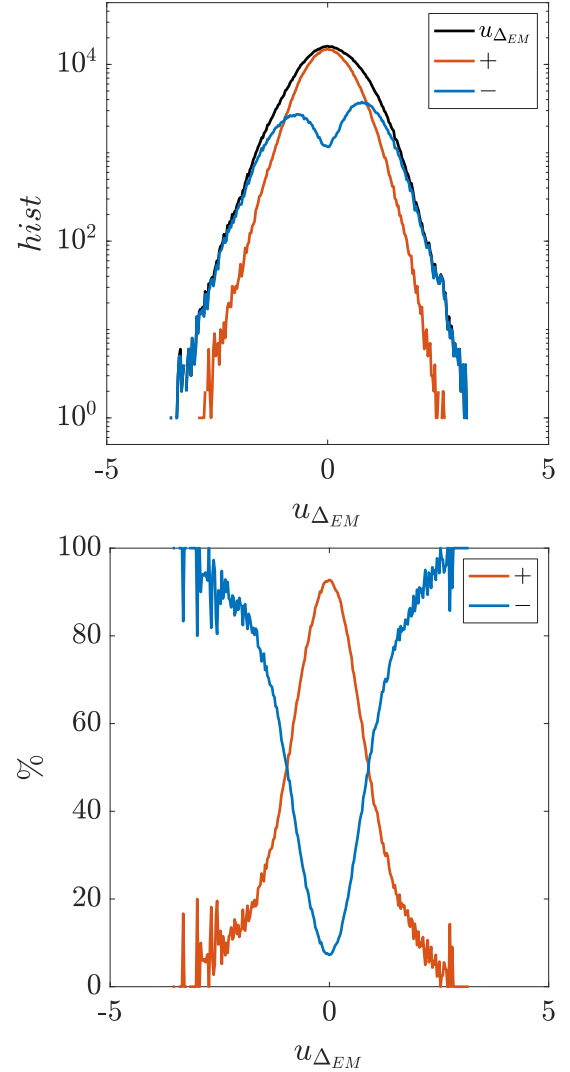
 Fig. 6: (a): Histogram of velocity increments without conditioning on entropy (black), condition on exclusively positive (red) and negative (blue) entropy trajectories are presented for  $u_{\Delta_{EM}}$ . (b): Percentage proportion in relation to the full (no condition) data set for positive and negative entropy condition.

In particular, it can be seen that the condition on positive entropy greatly reduces extreme increments at small scales, and nearly all ( $\approx 90\%$ ) of the large increments at small scales (heavy tailed statistics of the small-scale increment PDF) are contained in the negative entropy trajectories. Note, this could be seen as a new approach to the majority of large and intermittent small scale increments.

*Appendix F: Einstein-Markov time-scale for  $\mathbf{u}(\mathbf{x}_p, t)$ .*— In Fig. 7 the Markovian approximation is checked systematically for different values of  $\Delta\tau$ , using the Wilcoxon test for the fluid velocity at the particle position  $\mathbf{u}(\mathbf{x}_p, t)$ . Interestingly, the Einstein-Markov time-scale decreases with increasing St, unlike the behavior observed for  $\mathbf{v}(t)$ .

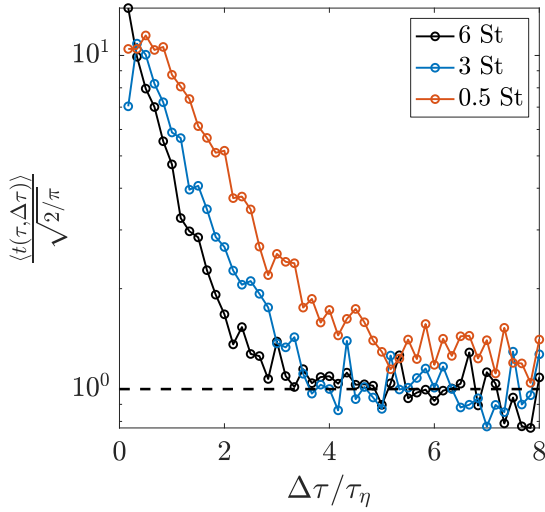

Fig. 7: Wilcoxon test for the particles trajectories: for the  $x$  component of the fluid velocity at the particle position  $\mathbf{u}(\mathbf{x}_p, t)$  for all Stokes numbers studied here as function of  $\Delta\tau$ . Note, that the normalized expectation value  $t(\tau, \Delta\tau)$  is supposed to be close to 1 if the Markovian assumption is valid (see [7, 11] and Appendix G for details and the description of essential notions).

*Appendix G: Essential notions.*— A central assumption of the Friedrich-Peinke approach is that the turbulent cascade process (more precisely the statistics of the scale-dependent velocity increments) possesses a Markov process. Experimental evidences show that the Markov property can be assumed to hold for the cascade coarse-grained by the Einstein-Markov coherence scale  $\Delta_{EM}$  [7, 11], which suggests that molecular friction causes the break-down of the Markov assumption, where the disorder of two increments are linked via memory effects, if the separation of scales is smaller than  $\Delta_{EM}$ . This finite step length can be seen in close analogy to the free mean path length of a Brownian diffusion process, which has to be so large, that two successive steps of the process can be considered as independent events [12]. For Markovian processes the relation  $p(u_{\tau_2}|u_{\tau_1}) = p(u_{\tau_2}|\dots, u_{\tau_1}, u_{\tau_0})$  holds. For finite

datasets,

$$p(u_{\tau_2}|u_{\tau_1}) = p(u_{\tau_2}|u_{\tau_1}, u_{\tau_0}), \quad (6)$$

is commonly assumed to be a sufficient condition. The Wilcoxon test is a parameter-free procedure to compare these two multi-scale statistics of velocity increments (two data sets of conditioned velocity increments). Therefore Eq. 6 is validated for the three different scales  $\tau_0 > \tau_1 > \tau_2$ , each separated by  $\Delta\tau = \Delta_{EM}$ . For this chosen set of scales the normalized expectation value  $\frac{\langle t(\tau, \Delta\tau) \rangle}{\sqrt{2/\pi}}$  of the number of inversions of the conditional velocity increment as a function of  $\Delta\tau$  is calculated. If the Markov properties holds the expectation value is equal to 1. A detailed description of the test is given in [7, 11].

## REFERENCES

- [1] GARDINER C. W., *Handbook of Stochastic Methods for physics, chemistry, and the natural sciences* 4th Edition (Springer, Berlin) 2009.
- [2] KLEINHANS D., FRIEDRICH R., NAWROTH A. and PEINKE J., *Physics Letters A*, **346** (2005) 42.
- [3] KLEINHANS D., *Physical Review E*, **85** (2012) 026705.
- [4] NAWROTH A. P., PEINKE J., KLEINHANS D. and FRIEDRICH R., *Physical Review E*, **76** (2007) 056102.
- [5] REINKE N., FUCHS A., NICKELSEN D. and PEINKE J., *Journal of Fluid Mechanics*, **848** (2018) 117.
- [6] RISKEN H., *Fokker-planck equation in The Fokker-Planck Equation* (Springer Berlin Heidelberg) 1996 pp. 63–95.
- [7] RENNER C., PEINKE J. and FRIEDRICH R., *Journal of Fluid Mechanics*, **433** (2001) 383.
- [8] RENNER C., PEINKE J., FRIEDRICH R., CHANAL O. and CHABAUD B., *Physical Review Letters*, **89** (2002) 124502.
- [9] FUCHS A., QUEIRÓS S. M. D., LIND P. G., GIRARD A., BOUCHET F., WÄCHTER M. and PEINKE J., *Physical Review Fluids*, **5** (2020) 034602.
- [10] FUCHS A., KHARCHÉ S., WÄCHTER M. and PEINKE J., *An open source matlab package for solving fokker-planck equation and validation of integral fluctuation theorem* [http://github.com/andre-fuchs-uni-oldenburg/open\\_fpe\\_ifft](http://github.com/andre-fuchs-uni-oldenburg/open_fpe_ifft).  
[https://github.com/andre-fuchs-uni-oldenburg/OPEN\\_FPE\\_IFT](https://github.com/andre-fuchs-uni-oldenburg/OPEN_FPE_IFT)
- [11] LUECK S., RENNER C., PEINKE J. and FRIEDRICH R., *Physics Letters A*, **359** (2006) 335.
- [12] EINSTEIN A., *Annalen der Physik*, **322** (1905) 549.
